# Supplementary material for: Co-training for On-board Deep Object Detection
Source: arXiv:2008.05534 source file (2020-08-12)
Supplement: Supplementary file 1 [file appendix.tex]

\begin{table}
\appendix
\centering
\caption{Summary of the symbols used in this paper, as well as specific abbreviations.}\label{tab:symbolsSummary}
\resizebox{1.0\linewidth}{!}{
\begin{tabular}{@{}ll@{}}
\toprule
Symbol & Meaning  \\
\toprule
a & b\\
\midrule
c & d\\
\bottomrule
\end{tabular}
}
\end{table}
